# Supplementary material for: Resolution analysis of magnetically arrested disk simulations
Source: arXiv:2405.00564 source file (2024-07-26)
Supplement: Supplementary file 1 [file Appendix.tex]

\appendix

\section{Jet funnel power}

Fig.~\ref{fig:Pj} shows the time averaged mass accretion rate and power ($P_{\mathrm{funnel}}\equiv\dot{M}_{\mathrm{funnel}}-\dot{E}_{\mathrm{funnel}}$) of the jet funnel ($\sigma>1$) as a function of radius. There is a significant contribution of matter accretion from both poles of the black hole, for radius $<5r_g$, due to density floors. At the event horizon, $\dot{M}$ reaches values up to $\approx 60$ in code units. For R2 and higher, jet power increases from approximately 20 to 30 in code units and converges from resolution R4. This may lead to an underestimation of the true jet power in low resolution simulations due to numerical floor contamination and magnetic energy dissipation along the vertical direction when the width of the polar axis is comparable to the width of the jet funnel. $P_{\mathrm{funnel}}$ is not exactly a measure of the Blandford Znajek power \citep{blandford1977electromagnetic}, because the cut $\sigma>1$ sometimes includes outflows from equatorial field lines.

%\op{I think GRMHD can accurately recover BZ already at low resolutions.  So this is probably not a matter of insufficient resolution for the induction + momentum equations.  Take away the disk (e.g. the monopole magnetosphere), and they will give the same power.  Could it have something to do with the opening angle of the jet and that you get more jet outflow from equatorial field lines?  Floor contamination should be visible in sigma, at z=20 they are all the same.}

\begin{figure}
	\includegraphics[width=\columnwidth]{Figures/Pjet_tavg.png}
    \caption{Jet funnel properties as a function of $z$, averaged in time $t=[8-10]\times 10^{3} r_g/c$. Mass accretion rate (top panel). Jet power (bottom panel). Positive/negative values of $\dot{M}_j$ mean inflow/outflow. Plus and minus the standard deviation is shown in dash-dotted lines for R1 and R5. The averaged values in radius $r=[5-1000]r_g$ is presented in the labels.}
    \label{fig:Pj}
\end{figure}

The EHTC adopted a lower limit on the jet power of $10^{42} \mathrm{erg/s}$ to constrain GRMHD models of \M87. They showed that most SANE models even with BH spin $ a = 0.94$ and some MAD models with $\left | a \right | \leqslant  0.5$ fail that constraint \citepalias{EHTC2019V,EHTC2021VIII}. In our simulations, the jet funnel power increases by a factor of 1,5 with resolution. This may lead to an underestimation of the true jet power in low resolution simulations. The alternative is the outflow power as a more reliable constraint from GRMHD simulations, which represents an upper bound of the jet power.
